# Supplementary material for: On the physisorption of water on graphene: Sub-chemical accuracy from many-body electronic structure methods
Source: arXiv:1811.07645 source file (2018-11-19)
Supplement: Supplementary file 1 [file suppinfo.pdf]

# Supporting Information

# On the physisorption of water on graphene: Sub-chemical accuracy from many-body electronic structure methods

Jan Gerit Brandenburg,[1,2] Andrea Zen,[1,2] Martin Fitzner,[1,2]
Benjamin Ramberger,[3] Georg Kresse,[3] Theodoros Tsatsoulis,[4]
Andreas Grüneis,[4] Angelos Michaelides,[1,2,*] and Dario Alfè[5,2,†]

[1]*Department of Physics and Astronomy,*
*University College London, Gower Street,*
*London WC1E 6BT, United Kingdom*

[2]*Thomas Young Centre and London Centre for Nanotechnology,*
*17-19 Gordon Street, London WC1H 0AH, United Kingdom*

[3]*University of Vienna, Faculty of Physics and*
*Center for Computational Materials Sciences,*
*Sensengasse 8/12, 1090 Wien, Austria*

[4]*Institute for Theoretical Physics, Vienna University of Technology,*
*Wiedner Hauptstrasse 8-10, 1040 Vienna,*
*Austria and Max Planck Institute for Solid State Research,*
*Heisenbergstrasse 1, 70569 Stuttgart, Germany*

[5]*Department of Earth Sciences, University College London,*
*Gower Street, London WC1E 6BT, United Kingdom*

(Dated: November 19, 2018)

* angelos.michaelides@ucl.ac.uk
† d.alfe@ucl.ac.uk

**CONTENTS**

S1. DMC setup: time step and population size S3

S2. L-CCSD(T) convergence S6

S3. Individual intercation energies S7

S4. Work function S11

S5. Interaction from density functional theory S11

S6. Symmetry adapted perturbation theory S13

References S15

## S1. DMC SETUP: TIME STEP AND POPULATION SIZE

The choice of the DMC setup, and in particular of the time step and walker population size, was tested carefully in a number or representative systems. The dependence of the evaluated DMC binding energy in terms of the time step size is reported in fig. S1, and in terms of the population bias in fig. S2.

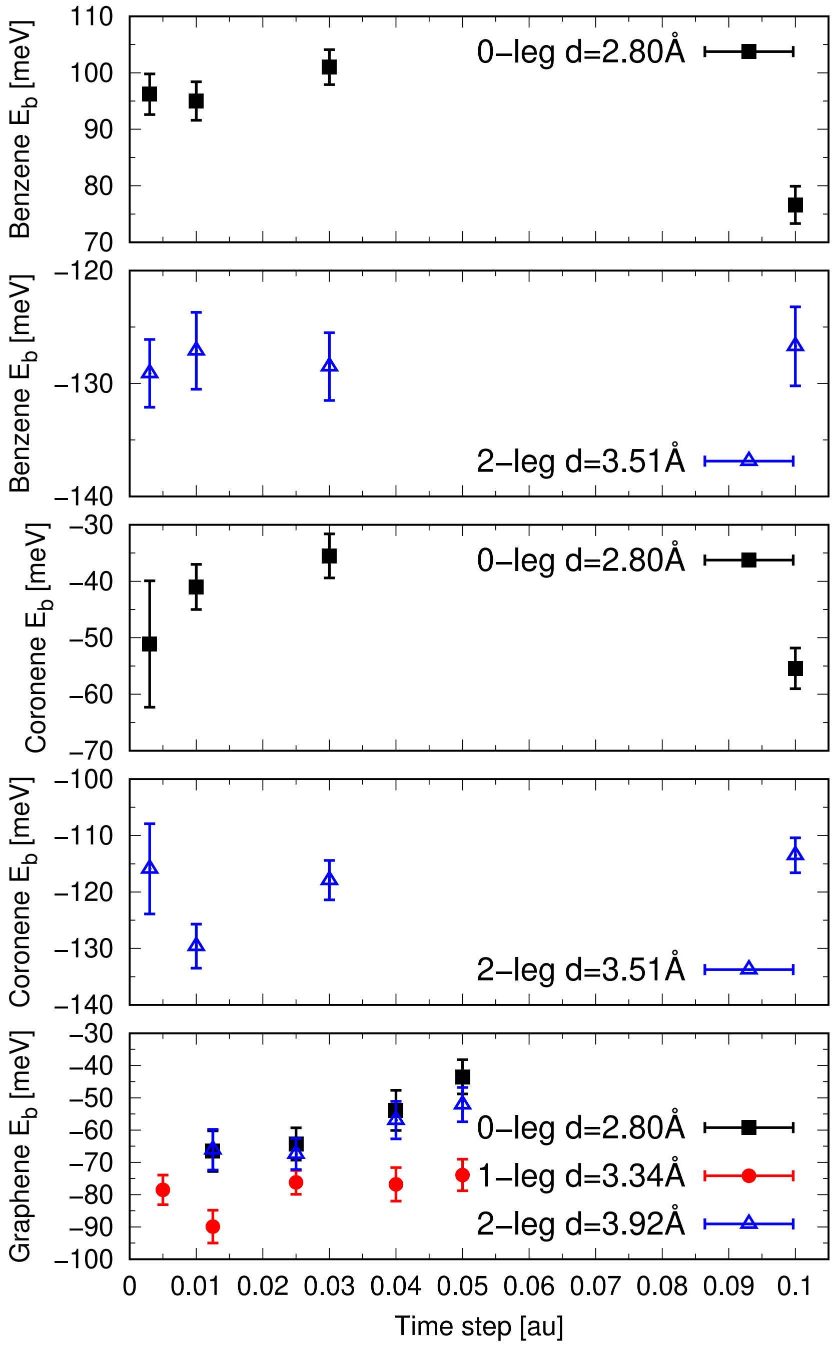


FIG. S1. DMC binding energy evaluation for water on benzene, coronene and graphene, reported as a function the DMC time step value. The plots show that the setup chosen to obtain the results reported in the main manuscript have a negligible bias due to finite time step errors.

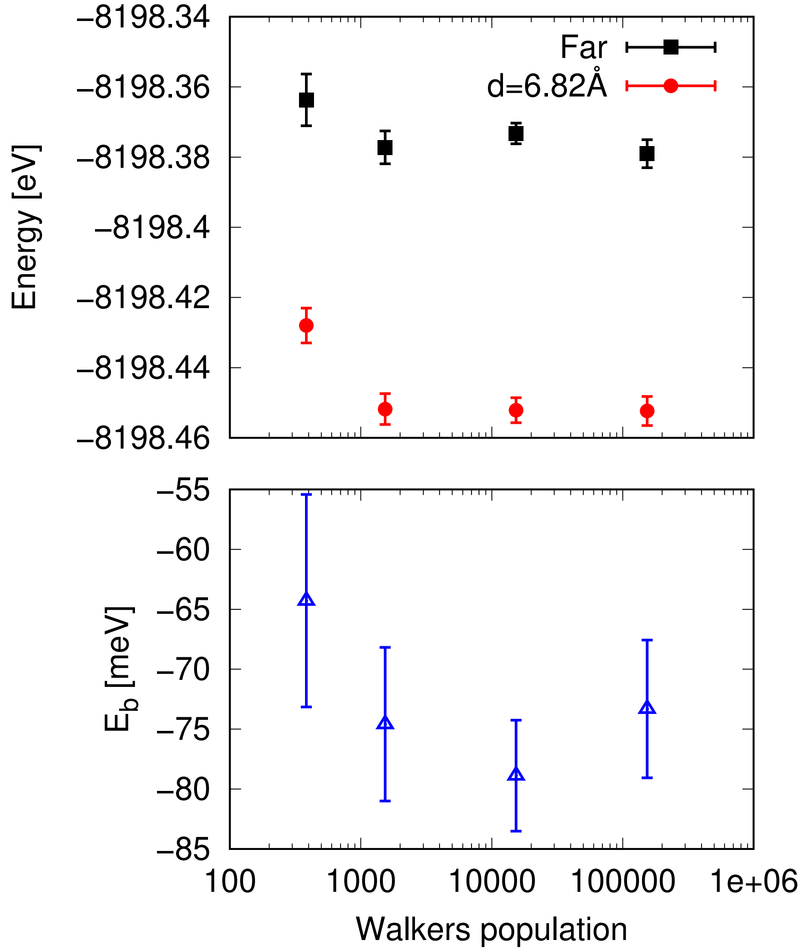


FIG. S2. Test of the population bias in DMC calculations for water on graphene, for the total energy (upper panel) and the binding energy $E_b$ (lower panel). The plots show that the setup chosen to obtain the results reported in the main manuscript have a negligible population bias.

## S2. L-CCSD(T) CONVERGENCE

TABLE S1. L-CCSD(T) binding energies for 0-leg ($d_{\mathrm{ads}} = 2.80\,\text{Å}$) and 2-leg ($d_{\mathrm{ads}} = 3.52\,\text{Å}$) adsorption on benzene separated into Hartree-Fock (HF) and correlation contribution $E_{\mathrm{corr}}$ calculated with increasingly large basis sets. Energies are given in meV, the finally used interaction energies are highlighted in bold.

| | HF | | $E_{\mathrm{corr}}$ | | $E_{\mathrm{tot}}$ | |
|---|---|---|---|---|---|---|
| | w.o.c.[a] | CP[b] | w.o.c. | CP | w.o.c. | CP |
| **0-leg** | | | | | | |
| cc-pVDZ | 257.63 | 316.30 | -140.70 | -107.39 | 116.93 | 208.91 |
| cc-pV(D/T)Z[c] | 193.89 | 296.92 | -322.30 | -158.71 | -128.41 | 138.21 |
| cc-pVTZ | 263.22 | 294.19 | -175.78 | -147.05 | 87.44 | 147.14 |
| cc-pVQZ | 276.14 | 288.94 | -181.68 | -168.27 | 94.46 | 120.67 |
| cc-pV5Z | 281.80 | 284.97 | -186.77 | -180.53 | 95.03 | 104.44 |
| CBS(4,5) | 283.96 | **283.46** | -191.99 | -193.11 | 91.97 | 90.35 |
| CBS+(4,5)[d] | – | – | -183.61 | -193.63 | 100.35 | 89.83 |
| CBS*(4,5)[e] | – | – | -184.15 | **-186.81** | 99.81 | **96.65** |
| **2-leg** | | | | | | |
| cc-pVDZ | -74.52 | -58.70 | -34.97 | -19.40 | -109.49 | -78.10 |
| cc-pV(D/T)Z[c] | -139.89 | -58.27 | -176.60 | -45.90 | -316.48 | -104.17 |
| cc-pVTZ | -82.03 | -52.55 | -73.95 | -52.40 | -155.98 | -104.95 |
| cc-pVQZ | -66.58 | -51.16 | -80.50 | -67.04 | -147.09 | -118.20 |
| cc-pV5Z | -54.55 | -50.05 | -79.87 | -74.18 | -134.42 | -124.23 |
| CBS(4,5) | -49.97 | **-49.63** | -79.21 | -81.67 | -129.18 | -131.30 |
| CBS+(4,5)[d] | – | – | -76.42 | -87.98 | -126.39 | -137.61 |
| CBS*(4,5)[e] | – | – | -77.48 | **-81.06** | -127.45 | **-130.69** |

[a] Plain interaction energy.
[b] Boys-Bernardi counterpoise corrected interaction energys.
[c] cc-pVDZ with modified exponents for carbon and aug-cc-pVTZ for hydrogen and oxygen atoms [1].
[d] Extrapolation using RPA correlation energies in the additive scheme.
[e] Extrapolation using RPA correlation energies in the multiplicative scheme.

## S3. INDIVIDUAL INTERCATION ENERGIES

TABLE S2. Adsorption energies $E_{ad}$ of single water monomer on benzene from DMC, L-CCSD(T), and RPA. Individual fragments are kept frozen for the evaluation of the intercation energy. The water-substrate distance $d_{ads}$ is defined according to Fig. 1, distances are given in Å and energies in meV.

| | DMC | | L-CCSD(T) | | RPA |
|---|---|---|---|---|---|
| $d_{ads}$ | $E_{ad}$ | $\sigma$[a] | $E_{ad}$ | $\Delta$CP[b] | $E_{ad}$ |
| **benzene, 0-leg motif** | | | | | |
| 2.237 | 676.0 | 3.1 | 635.8 | 3.9 | 634.6 |
| 2.516 | 265.4 | 3.1 | 249.0 | 2.4 | 248.9 |
| 2.796 | 92.8 | 3.4 | 96.7 | 1.6 | 96.5 |
| 3.075 | 42.1 | 4.5 | 43.3 | 1.2 | 43.1 |
| 3.355 | 25.3 | 4.2 | 28.4 | 0.9 | 27.4 |
| 4.194 | 22.6 | 3.3 | 22.0 | 0.1 | 22.5 |
| **benzene, 1-leg motif** | | | | | |
| 2.878 | 23.9 | 4.0 | 17.2 | 7.1 | 43.3 |
| 3.289 | -120.3 | 3.9 | -122.6 | 4.0 | -107.4 |
| 3.450 | – | – | – | – | -114.2 |
| 3.700 | -120.7 | 3.8 | -115.2 | 1.8 | -105.9 |
| 4.112 | -78.8 | 4.0 | -85.7 | 0.7 | -79.3 |
| 4.523 | -54.9 | 3.8 | -60.0 | 0.4 | -55.9 |
| 4.934 | -30.6 | 3.9 | -42.4 | 0.6 | -39.8 |
| 6.167 | -10.8 | 4.0 | -16.2 | 1.7 | -16.5 |
| **benzene, 2-leg motif** | | | | | |
| 2.805 | -3.6 | 4.4 | -1.8 | 5.6 | 18.8 |
| 3.155 | -128.8 | 4.5 | -129.1 | 3.3 | -114.8 |
| 3.320 | – | – | – | – | -125.5 |
| 3.506 | -129.4 | 3.4 | -130.7 | 1.6 | -121.5 |
| 3.856 | -104.1 | 3.3 | -103.8 | 0.2 | -97.8 |
| 4.207 | -74.7 | 3.1 | -78.1 | 1.2 | -73.0 |
| 5.259 | -34.5 | 4.0 | -32.0 | 1.9 | -30.8 |

[a] Stochastic DMC error.

[b] We report half the size of the CP correction $\Delta$ as an indicator for basis set convergence.

TABLE S3. Adsorption energies $E_{ad}$ of single water monomer on coronene from DMC, L-CCSD(T), and RPA. Individual fragments are kept frozen for the evaluation of the intercation energy. The water-substrate distance $d_{ads}$ is defined according to Fig. 1, distances are given in Å and energies in meV.

| | DMC | | L-CCSD(T) | | RPA |
|---|---|---|---|---|---|
| $d_{ads}$ | $E_{ad}$ | $\sigma$[a] | $E_{ad}$ | $\Delta$CP[b] | $E_{ad}$ |
| **coronene, 0-leg motif** | | | | | |
| 2.237 | – | – | 347.8 | 11.0 | 363.5 |
| 2.516 | – | – | 50.4 | 7.4 | 65.5 |
| 2.796 | -46.5 | 4.0 | -45.9 | 5.1 | -32.5 |
| 3.075 | -58.4 | 4.0 | -60.0 | 3.4 | -49.5 |
| 3.355 | -46.7 | 4.2 | -51.0 | 1.2 | -39.8 |
| 4.194 | – | – | -10.6 | 1.8 | -1.3 |
| **coronene, 1-leg motif** | | | | | |
| 2.878 | 34.6 | 4.3 | 25.1 | 10.4 | 59.4 |
| 3.289 | -112.4 | 3.9 | -115.3 | 5.9 | -91.6 |
| 3.450 | – | – | – | na | -109.8 |
| 3.700 | -102.5 | 3.7 | -111.9 | 2.6 | -93.2 |
| 4.112 | -83.5 | 3.9 | -86.0 | 1.9 | -70.1 |
| 4.523 | – | – | -63.1 | 0.9 | -49.8 |
| 4.934 | – | – | -46.1 | 0.7 | -35.4 |
| 6.167 | – | – | -20.7 | 2.4 | -13.5 |
| **coronene, 2-leg motif** | | | | | |
| 2.805 | – | – | -27.8 | 11.0 | 5.5 |
| 3.155 | -131.9 | 4.0 | -137.9 | 7.4 | -115.8 |
| 3.320 | – | – | – | – | -125.5 |
| 3.506 | -135.1 | 3.9 | -138.9 | 3.8 | -122.3 |
| 3.856 | -104.0 | 4.3 | -115.8 | 0.9 | -101.5 |
| 4.207 | – | – | -91.8 | 1.4 | -79.5 |
| 5.259 | – | – | -46.5 | 2.7 | -40.9 |

[a] Stochastic DMC error.

[b] We report half the size of the CP correction $\Delta$ as an indicator for basis set convergence.

TABLE S4. Adsorption energies $E_{ad}$ of single water monomer on graphene (0-leg and 1-leg motif) from DMC, RPA, and RPA+GWSE. Individual fragments are kept frozen for the evaluation of the intercation energy. The water-substrate distance $d_{ads}$ is defined according to Fig. 1, distances are given in Å and energies in meV.

| | DMC | | RPA | RPA+GWSE |
|---|---|---|---|---|
| $d_{ads}$ | $E_{ad}$ | $\sigma$[a] | $E_{ad}$ | $E_{ad}$ |
| **graphene, 0-leg motif** | | | | |
| 2.266 | – | – | 296.4 | 263.0 |
| 2.531 | 23.5 | 6.6 | 32.0 | 11.4 |
| 2.597 | -4.9 | 6.2 | – | – |
| 2.663 | -33.3 | 5.8 | -27.9 | -44.4 |
| 2.730 | -60.9 | 5.7 | – | – |
| 2.796 | -76.0 | 5.0 | -60.9 | -74.5 |
| 3.060 | -84.4 | 5.6 | -80.8 | -89.7 |
| 3.325 | -72.3 | 5.7 | -74.1 | -80.3 |
| 3.590 | -69.8 | 5.7 | -59.5 | -63.8 |
| 3.854 | -60.5 | 5.7 | -46.5 | -49.3 |
| 4.383 | -41.7 | 6.5 | -26.7 | -28.1 |
| 4.912 | -17.3 | 5.7 | – | – |
| 5.442 | -9.2 | 6.5 | – | – |
| 5.971 | -2.6 | 5.9 | -9.9 | -9.8 |
| 6.500 | -6.8 | 8.0 | – | – |
| 6.970 | – | – | -9.2 | -8.9 |
| **graphene, 1-leg motif** | | | | |
| 2.900 | 48.6 | 5.3 | 81.4 | 43.7 |
| 3.016 | -26.6 | 5.8 | 10.6 | -20.2 |
| 3.164 | -70.6 | 5.9 | -41.1 | -65.1 |
| 3.339 | -83.5 | 4.7 | -68.8 | -85.4 |
| 3.609 | -87.1 | 4.6 | -71.1 | -82.8 |
| 3.874 | -84.9 | 5.8 | -60.9 | -68.5 |
| 4.112 | -53.9 | 5.8 | -48.2 | -53.4 |
| 4.583 | -25.9 | 7.4 | -29.0 | -31.5 |
| 5.207 | -18.9 | 4.9 | -16.3 | -17.1 |
| 6.064 | -2.7 | 5.1 | -9.1 | -8.9 |
| 7.276 | -0.8 | 5.2 | -6.8 | -6.4 |

[a] Stochastic DMC error.

TABLE S5. Adsorption energies $E_{\mathrm{ad}}$ of single water monomer on graphene (2-leg motif) from DMC, RPA, and RPA+GWSE. Individual fragments are kept frozen for the evaluation of the intercation energy. The water-substrate distance $d_{\mathrm{ads}}$ is defined according to Fig. 1, distances are given in Å and energies in meV.

| | DMC | | | RPA | RPA+GWSE |
|---|---|---|---|---|---|
| $d_{\mathrm{ads}}$ | $E_{\mathrm{ad}}$ | $\sigma$[a] | $d_{\mathrm{ads}}$ | $E_{\mathrm{ad}}$ | $E_{\mathrm{ad}}$ |
| **graphene, 2-leg motif** | | | | | |
| 2.712 | 104.7 | 6.2 | 2.79 | 73.3 | 31.7 |
| 2.977 | -49.2 | 6.1 | 2.99 | -31.5 | -61.4 |
| 3.241 | -95.6 | 6.1 | 3.09 | -57.8 | -83.3 |
| 3.506 | -98.4 | 5.7 | 3.19 | -71.6 | -93.3 |
| 3.770 | -75.6 | 5.9 | 3.39 | -80.7 | -96.6 |
| 3.925 | -74.2 | 4.8 | 3.59 | -75.9 | -87.6 |
| 4.300 | -49.8 | 5.8 | 3.92 | -58.6 | -65.5 |
| 4.829 | -27.7 | 6.0 | 4.26 | -42.1 | -46.2 |
| 5.358 | -14.3 | 6.5 | 5.26 | -16.3 | -16.9 |
| 5.887 | -0.6 | 6.7 | 6.2 | -9.3 | -8.9 |
| 6.416 | 3.9 | 6.3 | – | – | – |

[a] Stochastic DMC error.

## S4. WORK FUNCTION

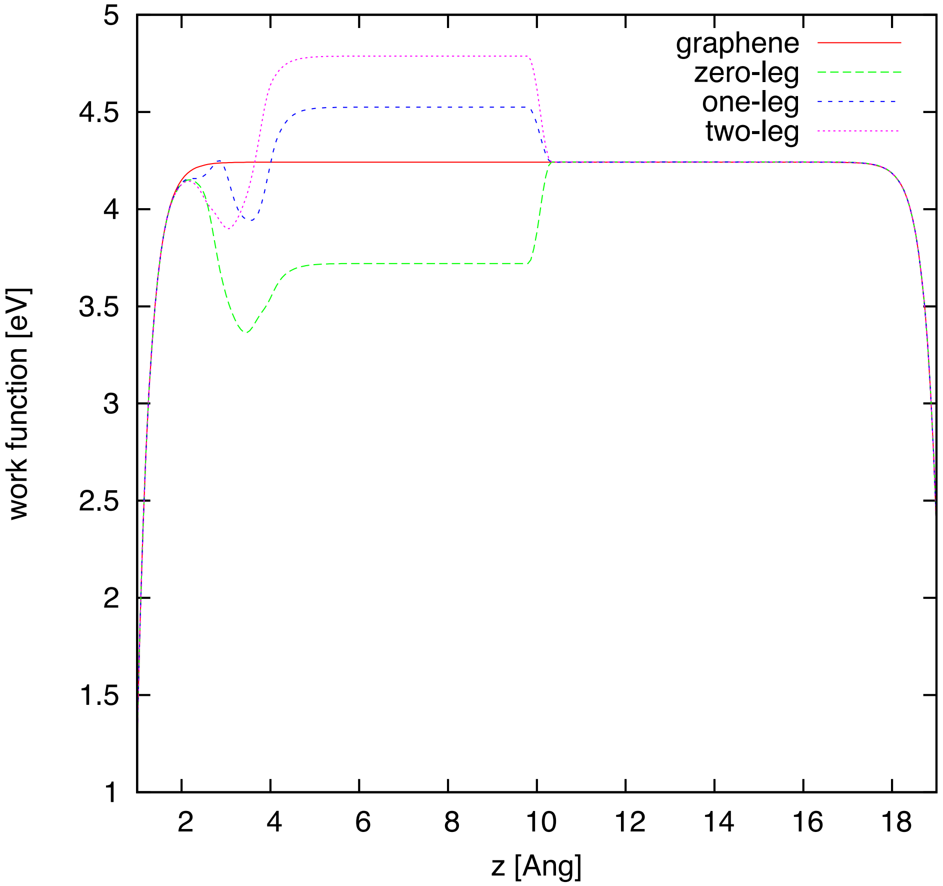


FIG. S3. DFT based workfunction for a single graphene layer and the adsorbed water monomer in the 0-leg, 1-leg, and 2-leg configuration.

## S5. INTERACTION FROM DENSITY FUNCTIONAL THEORY

TABLE S6. Benchmarking several dispersion corrected DFAs for the water adsorption energy on graphene compared to DMC references [meV].

| | graphene[a] | | | | | cluster[b] |
|---|---|---|---|---|---|---|
| | 0-leg | 1-leg | 2-leg | $\Delta_{\mathrm{min}}^{\mathrm{max}\,c}$ | MUE | MUE |
| DMC | -90±6 | -92±6 | -99±6 | 9±6 | – | – |
| RPA | -81 | -74 | -82 | 8 | 15 | 7 |
| RPA+GWSE | -90 | -87 | -98 | 11 | 2 | – |
| PBE[2] | -8 | -22 | -20 | 14 | 77 | 65 |
| PBE-D2[2, 3] | -88 | -124 | -137 | 49 | 24 | 15 |
| **PBE-D3**[2, 4][d] | -84 | -113 | -125 | 41 | **18** | **8** |
| **PBE-D4**[2, 5] | -103 | -109 | -117 | 14 | **16** | **4** |
| PBE-TS[2, 6] | -115 | -137 | -161 | 46 | 44 | 20 |
| **PBE-MBD**[2, 7] | -93 | -116 | -127 | 34 | **18** | **7** |
| PBE-dDsC[2, 8] | -104 | -123 | -138 | 34 | 28 | 12 |
| PBE-VV10[2, 9] | -122 | -126 | -140 | 18 | 36 | 21 |
| SCAN[10] | -62 | -79 | -82 | 20 | 19 | 13 |
| vdW-DF1[11] | -136 | -131 | -135 | 5 | 40 | 20 |
| optB88-vdW[12] | -139 | -138 | -150 | 21 | 49 | 19 |
| vdW-DF2[13] | -128 | -126 | -134 | 6 | 36 | 16 |
| **rev-vdW-DF2**[14] | -105 | -106 | -118 | 13 | **16** | **7** |
| HF | 37 | 21 | 60 | 39 | 133 | 130 |
| HF-D4 | -107 | -110 | -87 | 23 | 28 | 24 |
| **PBE0-D4**[5, 15] | -102 | -110 | -107 | 8 | **13** | **3** |
| **PBE0-MBD**[7, 15] | -87 | -112 | -112 | 25 | **12** | **10** |
| sHF-3c[16, 17] | -67 | -83 | -117 | 50 | 17 | 23 |
| HSE-3c[18] | -123 | -106 | -128 | 12 | 25 | 37 |
| B97-3c[19] | -160 | -139 | -140 | 20 | 53 | 24 |
| DFTB3-D3[20–23] | -81 | -112 | -125 | 44 | 18 | 9 |
| GFN2-xTB[24] | -73 | -81 | -91 | 18 | 12 | 27 |

[a] Energies computed on fixed geometries, distance $d_{\mathrm{ads}}$ taken as DMC equilibrium value, see Table II, geometries given as Supporting Information files.

[b] MUEs on the benzene and coronene adsorptions compared to DMC references (6 binding energies).

[c] Difference between strongest and weakest adsorption motif.

[d] Best performing methods with MUE on clusters below 10 meV are highlighted in bold.

## S6. SYMMETRY ADAPTED PERTURBATION THEORY

As a means for partitioning the noncovalent interaction energy, we use symmetry adapted perturbation theory (SAPT [25–28]). We use the scaled SAPT0 in an aug-cc-pVDZ orbital expansion as implemented in PSI4 [29] and given by the energy expression

$$E_{\mathrm{SAPT0}} = E^{(10)}_{\mathrm{exch}} + E^{(10)}_{\mathrm{es}} + E^{(20)}_{\mathrm{ind}} + E^{(20)}_{\mathrm{disp}}\,, \tag{1}$$

where orbital relaxation effects are included and induction and dispersion energies include the exchange contributions [30]. It's fortunate error compensation has been shown on several test sets of molecular dimers [31]. For quantitative interaction energies higher order terms are necessary, which has been shown on large molecular complexes [32]. However, SAPT0 is specifically not used to compute reliable binding energies, but rather for a qualitative understanding of the involved interactions. In Fig. S4, we give the exchange repulsion $E_{EXR}$, electrostatic $E_{ES}$, induction $E_{ind}$, and dispersion $E_{disp}$ contributions for the water adsorption on benzene and coronene. Though we only analyze qualitative contributions, we note that total SAPT0 binding energies agree well with L-CCSD(T) data. The decreasing exchange-repulsion with larger substrate indicates that the electron density perpendicular to the substrate plane extends less, which partially confirms the charge density analysis. We can additionally confirm that electrostatic interactions are repulsive for the 0-leg configuration on benzene, while the 1-leg and 2-leg configurations are stabilized by electrostatics. The 0-leg electrostatic contribution is negligible for adsorption on coronene and we can estimate an attractive contribution for larger substrates. In contrast, the 1-leg and 2-leg electrostatic attraction decreases from adsorption on benzene to adsorption on coronene. Induction (including exchange induction) is attractive for all systems and slightly larger for the 1-leg and 2-leg motifs. Dispersion attraction is very similar for all binding motifs, the 2-leg contribution is stabilized most, and the contribution grows with increasing substrate size. Higher order many-body dispersion contributions are not covered at this SAPT0 level. We can overall conclude from this analysis that 1-leg and 2-leg adsorptions behave very similar, while 0-leg adsorption has a quite distinct electrostatic interaction going in hand with a pronounced charge reorganization in the substrate in order to have a competitive binding energy.

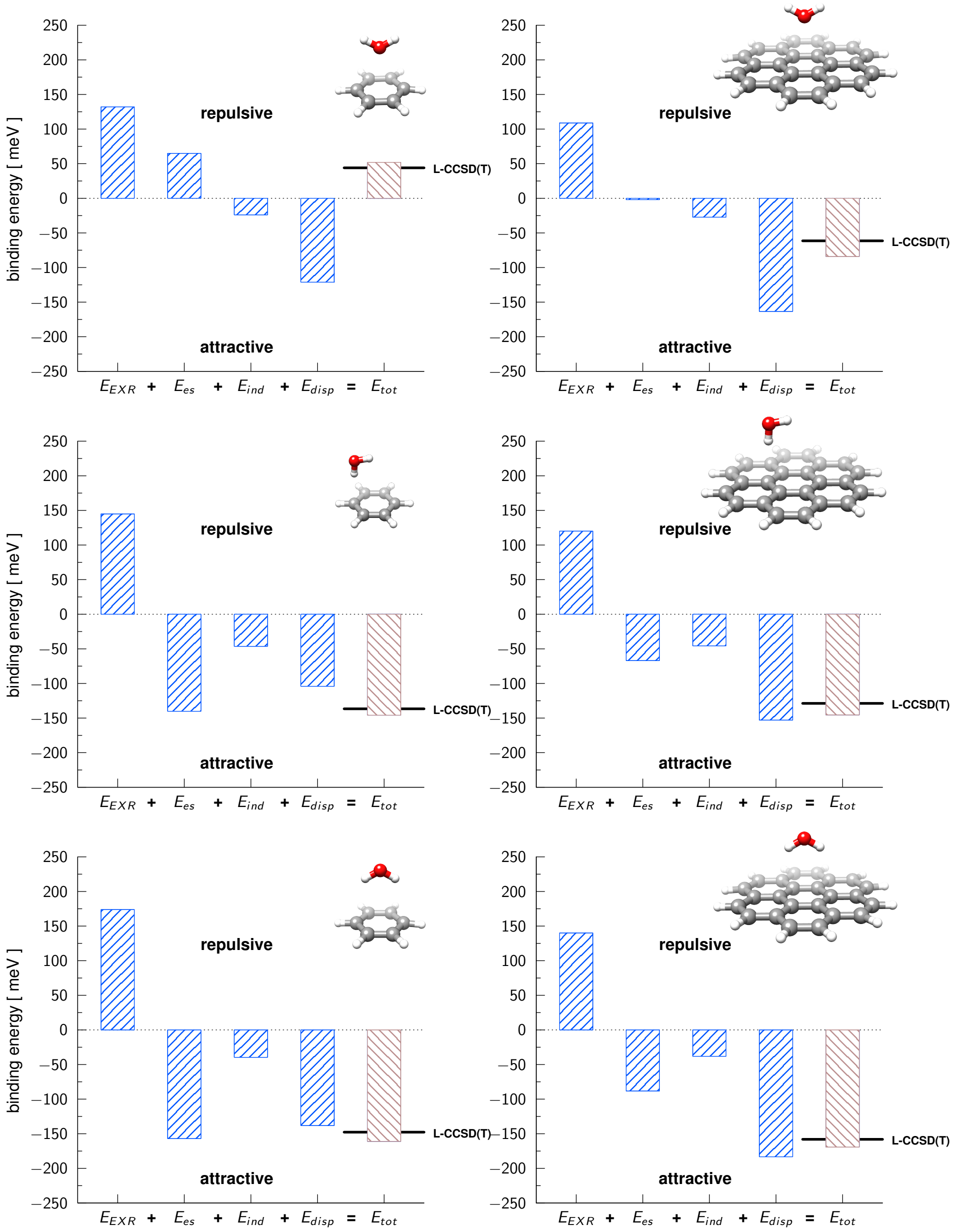


FIG. S4. SAPT energy partitioning for water@benzene and water@coronene (0-leg, 1-leg and 2-leg configurations) at equilibrium geometry. $E_{ind}$ and $E_{disp}$ include Coulomb and exchange contributions.

[1] E. Voloshina, D. Usvyat, M. Schutz, Y. Dedkov, and B. Paulus, Phys. Chem. Chem. Phys. **13**, 12041 (2011).

[2] J. P. Perdew, K. Burke, and M. Ernzerhof, Phys. Rev. Lett. **77**, 3865 (1996), erratum *Phys. Rev. Lett.* **78**, 1396 (1997).

[3] S. Grimme, J. Comput. Chem. **27**, 1787 (2006).

[4] S. Grimme, J. Antony, S. Ehrlich, and H. Krieg, J. Chem. Phys. **132**, 154104 (2010).

[5] DFT-D4 model will be published elsewhere. It is based on Ref. [33] and includes all dipole many-body orders.

[6] A. Tkatchenko and M. Scheffler, Phys. Rev. Lett. **102**, 073005 (2009).

[7] A. Tkatchenko, R. A. DiStasio., R. Car, and M. Scheffler, Phys. Rev. Lett. **108**, 236402 (2012).

[8] S. N. Steinmann and C. A. Corminboeuf, J. Chem. Theory Comput. **6**, 1990 (2010).

[9] O. A. Vydrov and T. Van Voorhis, J. Chem. Phys. **133**, 244103 (2010).

[10] J. Sun, A. Ruzsinszky, and J. P. Perdew, Phys. Rev. Lett. **115**, 036402 (2015).

[11] M. Dion, H. Rydberg, E. Schröder, D. C. Langreth, and B. I. Lundqvist, Phys. Rev. Lett. **92**, 246401 (2004).

[12] J. Klimeš, D. R. Bowler, and A. Michaelides, J. Phys.: Condens. Matter **22**, 022201 (2010).

[13] K. Lee, E. D. Murray, L. Kong, B. I. Lundqvist, and D. C. Langreth, Phys. Rev. B **82**, 081101 (2010).

[14] I. Hamada, Phys. Rev. B **89**, 121103(R) (2014).

[15] C. Adamo and V. Barone, J. Chem. Phys. **110**, 6158 (1999).

[16] R. Sure and S. Grimme, J. Comput. Chem. **34**, 1672 (2013).

[17] M. Cutini, B. Civalleri, M. Corno, R. Orlando, J. G. Brandenburg, L. Maschio, and P. Ugliengoa, J. Chem. Theory Comput. **12**, 3340 (2016).

[18] J. G. Brandenburg, E. Caldeweyher, and S. Grimme, Phys. Chem. Chem. Phys. **18**, 15519 (2016).

[19] J. G. Brandenburg, C. Bannwarth, A. Hansen, and S. Grimme, J. Chem. Phys. **148**, 064104 (2018).

[20] M. Elstner, D. Porezag, G. Jungnickel, J. Elsner, M. Haugk, T. Frauenheim, S. Suhai, and G. Seifert, Phys. Rev. B **58**, 7260 (1998).

[21] B. Aradi, B. Hourahine, and T. Frauenheim, J. Phys. Chem. A **111**, 5678 (2007).

[22] M. Gaus, A. Goez, and M. Elstner, J. Chem. Theory Comput. **9**, 338 (2013).

[23] J. G. Brandenburg and S. Grimme, J. Phys. Chem. Lett. **5**, 1785 (2014).

[24] S. Grimme, C. Bannwarth, and P. Shushkov, J. Chem. Theory Comput. **13**, 1989 (2017).

[25] E. G. Hohenstein and C. D. Sherrill, J. Chem. Phys. **132**, 184111 (2010).

[26] A. Heßelmann, G. Jansen, and M. Schütz, J. Chem. Phys. **122**, 014103 (2005).

[27] G. Jansen, WIREs Comput. Mol. Sci. **4**, 127 (2014).

[28] K. Szalewicz, WIREs Comput. Mol. Sci. **2**, 254 (2012).

[29] R. M. Parrish, L. A. Burns, D. G. A. Smith, A. C. Simmonett, A. E. DePrince, E. G. Hohenstein, U. Bozkaya, A. Y. Sokolov, R. Di Remigio, R. M. Richard, J. F. Gonthier, A. M. James, H. R. McAlexander, A. Kumar, M. Saitow, X. Wang, B. P. Pritchard, P. Verma, H. F. Schaefer, K. Patkowski, R. A. King, E. F. Valeev, F. A. Evangelista, J. M. Turney, T. D. Crawford, and C. D. Sherrill, J. Chem. Theory. Comput. **13**, 3185 (2017).

[30] B. Jeziorski, R. Moszynski, and K. Szalewicz, Chem. Rev. **94**, 1887 (1994).

[31] T. M. Parker, L. A. Burns, R. M. Parrish, A. G. Ryno, and C. D. Sherrill, J. Chem. Phys. **140**, 094106 (2014).

[32] A. Heßelmann and T. Korona, J. Chem. Phys. **141**, 094107 (2014).

[33] E. Caldeweyher, C. Bannwarth, and S. Grimme, J. Chem. Phys. **147**, 034112 (2017).
